# Supplementary material for: M-STAR: Multi-Scale Spatiotemporal Autoregression for Human Mobility Modeling
Source: arXiv:2512.07314 source file (2025-12-08)
Supplement: Supplementary file 1 [file X1_appendix.tex]

\setcounter{equation}{0}%将公式编号归0

\section{Appendix}
